# Supplementary material for: On binomial coefficients modulo squares of primes
Source: arXiv:1712.02095 ancillary file (2018-10-08)
Supplement: Supplementary file 1 [file lucascong-compiled.pdf]

# The Lucas and Babbage congruences

Darij Grinberg

October 7, 2018

## Contents

|                                                                        |           |
|------------------------------------------------------------------------|-----------|
| 0.1. Introduction . . . . .                                            | 1         |
| <b>1. The congruences</b>                                              | <b>2</b>  |
| 1.1. Binomial coefficients . . . . .                                   | 2         |
| 1.2. Negative $n$ . . . . .                                            | 3         |
| 1.3. The two congruences . . . . .                                     | 4         |
| <b>2. Proofs</b>                                                       | <b>5</b>  |
| 2.1. Basic properties of binomial coefficients modulo primes . . . . . | 5         |
| 2.2. Restating Vandermonde convolution . . . . .                       | 6         |
| 2.3. The congruence lemma . . . . .                                    | 9         |
| 2.4. Proof of the Lucas theorem . . . . .                              | 13        |
| 2.5. Two lemmas for Babbage's theorem . . . . .                        | 16        |
| 2.6. Proof of Babbage's theorem . . . . .                              | 17        |
| <b>3. The sums of the first <math>p</math> powers</b>                  | <b>19</b> |
| 3.1. The congruence . . . . .                                          | 19        |
| 3.2. Powers and power sums via Stirling numbers of the second kind . . | 20        |
| 3.3. Finishing the proof . . . . .                                     | 28        |

## 0.1. Introduction

In this expository note, we prove the Lucas and Babbage congruences for binomial coefficients. The proof is elementary (by induction) and functions for arbitrary integer parameters (as opposed to merely for nonnegative integers). Afterwards,

we also prove the congruence  $\sum_{l=0}^{p-1} l^k \equiv 0 \pmod{p}$  for any prime  $p$  and any  $k \in \mathbb{N}$  that is not a positive multiple of  $p$ .

# 1. The congruences

## 1.1. Binomial coefficients

Let us first recall the standard definition of binomial coefficients:<sup>1</sup>

**Definition 1.1.** Let  $n \in \mathbb{N}$  and  $m \in \mathbb{Q}$ . Then, the *binomial coefficient*  $\binom{m}{n}$  is a rational number defined by

$$\binom{m}{n} = \frac{m(m-1)\cdots(m-n+1)}{n!}.$$

This definition is precisely [Grinbe17, Definition 3.1].

The following properties of binomial coefficients are well-known and appear in [Grinbe17]:

**Proposition 1.2.** We have

$$\binom{m}{0} = 1 \tag{1}$$

for every  $m \in \mathbb{Q}$ .

Proposition 1.2 is [Grinbe17, Proposition 3.3 (a)].

**Proposition 1.3.** We have

$$\binom{m}{n} = 0 \tag{2}$$

for every  $m \in \mathbb{N}$  and  $n \in \mathbb{N}$  satisfying  $m < n$ .

Proposition 1.3 is [Grinbe17, Proposition 3.6].

**Proposition 1.4.** We have

$$\binom{m}{m} = 1 \tag{3}$$

for every  $m \in \mathbb{N}$ .

Proposition 1.4 is [Grinbe17, Proposition 3.9].

**Proposition 1.5.** We have

$$\binom{m}{n} = \binom{m-1}{n-1} + \binom{m-1}{n} \tag{4}$$

for any  $m \in \mathbb{Z}$  and  $n \in \{1, 2, 3, \dots\}$ .

---

<sup>1</sup>We use the notation  $\mathbb{N}$  for the set  $\{0, 1, 2, \dots\}$ .

Proposition 1.5 is a particular case of [Grinbe17, Proposition 3.11].

**Proposition 1.6.** We have  $\binom{m}{n} \in \mathbb{Z}$  for any  $m \in \mathbb{Z}$  and  $n \in \mathbb{N}$ .

Proposition 1.6 is [Grinbe17, Proposition 3.20].

**Proposition 1.7.** For every  $x \in \mathbb{Z}$  and  $y \in \mathbb{Z}$  and  $n \in \mathbb{N}$ , we have

$$\binom{x+y}{n} = \sum_{k=0}^n \binom{x}{k} \binom{y}{n-k}.$$

Proposition 1.7 is the so-called *Vandermonde convolution identity*, and is a particular case of [Grinbe17, Theorem 3.29].

## 1.2. Negative $n$

We have so far defined the binomial coefficient  $\binom{m}{n}$  only for  $n \in \mathbb{N}$ . For the sake of convenience, let us extend the definition of  $\binom{m}{n}$  to arbitrary integers  $n$ . To do so, we need to define  $\binom{m}{n}$  when  $n$  is a **negative** integer. We do so in the simplest possible way:

**Definition 1.8.** Let  $n$  be a negative integer. Let  $m \in \mathbb{Z}$ . Then, the *binomial coefficient*  $\binom{m}{n}$  is a rational number defined by  $\binom{m}{n} = 0$ .

This convention is the one used by Graham, Knuth and Patashnik in [GrKnPa]. Other authors use other conventions.

Hence, the binomial coefficient  $\binom{m}{n}$  is defined for all  $m \in \mathbb{Z}$  and  $n \in \mathbb{Z}$ . (Namely, it is defined in Definition 1.8 when  $n$  is negative, and it is defined in Definition 1.1 when  $n$  is nonnegative.)

The following fact is easy:

**Proposition 1.9.** We have  $\binom{m}{n} \in \mathbb{Z}$  for any  $m \in \mathbb{Z}$  and  $n \in \mathbb{Z}$ .

*Proof of Proposition 1.9.* When  $n$  is negative, Proposition 1.9 follows from  $\binom{m}{n} = 0$ . Thus, we WLOG assume that  $n$  is nonnegative. Hence,  $n \in \mathbb{N}$ . Thus, Proposition 1.9 follows from Proposition 1.6.  $\square$

We can also extend Proposition 1.5 to arbitrary integer values of  $n$ :

**Proposition 1.10.** We have

$$\binom{m}{n} = \binom{m-1}{n-1} + \binom{m-1}{n}$$

for any  $m \in \mathbb{Z}$  and  $n \in \mathbb{Z}$ .

*Proof of Proposition 1.10.* Let  $m \in \mathbb{Z}$  and  $n \in \mathbb{Z}$ . We are in one of the following three cases:

Case 1: We have  $n < 0$ .

Case 2: We have  $n = 0$ .

Case 3: We have  $n > 0$ .

Let us first consider Case 1. In this case, we have  $n < 0$ . Thus, both  $n$  and  $n - 1$  are negative integers. Hence, all three binomial coefficients  $\binom{m}{n}$ ,  $\binom{m-1}{n-1}$  and  $\binom{m-1}{n}$  equal 0 (by Definition 1.8). Therefore, the claim of Proposition 1.10 rewrites as  $0 = 0 + 0$ , which is clearly true. Thus, Proposition 1.10 is proven in Case 1.

Let us next consider Case 2. In this case, we have  $n = 0$ . Hence,  $n - 1 = -1$  is a negative integer. Therefore, Definition 1.8 yields  $\binom{m-1}{n-1} = 0$ . Also, from  $n = 0$ , we obtain  $\binom{m}{n} = \binom{m}{0} = 1$  and  $\binom{m-1}{n} = \binom{m-1}{0} = 1$ . Hence,

$$\underbrace{\binom{m-1}{n-1}}_{=0} + \underbrace{\binom{m-1}{n}}_{=1} = 1.$$

Comparing this with  $\binom{m}{n} = 1$ , we obtain  $\binom{m}{n} = \binom{m-1}{n-1} + \binom{m-1}{n}$ . Thus, Proposition 1.10 is proven in Case 2.

Let us finally consider Case 3. In this case, we have  $n > 0$ . Thus,  $n \in \{1, 2, 3, \dots\}$ . Hence, Proposition 1.5 yields  $\binom{m}{n} = \binom{m-1}{n-1} + \binom{m-1}{n}$ . Thus, Proposition 1.10 is proven in Case 3.

We have now proven Proposition 1.10 in each of the three Cases 1, 2 and 3. This completes the proof.  $\square$

### 1.3. The two congruences

Proposition 1.9 shows that  $\binom{m}{n}$  is an integer whenever  $m \in \mathbb{Z}$  and  $n \in \mathbb{Z}$ . We shall use this fact tacitly. It allows us to state congruences involving binomial coefficients.

Next, let us state two classical results on the behavior of binomial coefficients modulo primes:

**Theorem 1.11.** Let  $p$  be a prime. Let  $a$  and  $b$  be two integers. Let  $c$  and  $d$  be two elements of  $\{0, 1, \dots, p-1\}$ . Then,

$$\binom{ap+c}{bp+d} \equiv \binom{a}{b} \binom{c}{d} \pmod{p}.$$

Theorem 1.11 is known under the name of *Lucas's theorem*, and is proven in many places (e.g., [Mestro14, §2.1] or [Hausne83, Proof of §4] or [AnBeRo05, proof of Lucas's theorem] or [GrKnPa, Exercise 5.61]) in the case when  $a$  and  $b$  are nonnegative integers. The standard proof of Theorem 1.11 in this case uses generating functions; it is not hard to tweak this proof so that it applies (*mutatis mutandis*) in the general case as well. But we are going to give a different, more elementary proof of Theorem 1.11.

Another classical result about binomial coefficients and primes is the following fact:

**Theorem 1.12.** Let  $p$  be a prime. Let  $a$  and  $b$  be two integers. Then,

$$\binom{ap}{bp} \equiv \binom{a}{b} \pmod{p^2}.$$

In the case when  $a$  and  $b$  are nonnegative integers, Theorem 1.12 is a known result, due to Charles Babbage (see, e.g., [Stan11, Exercise 1.14 c] or [GrKnPa, Exercise 5.62]). Notice that if  $p \geq 5$ , then the modulus  $p^2$  can be replaced by  $p^3$  or (depending on  $a$ ,  $b$  and  $p$ ) by even higher powers of  $p$ ; see [Mestro14, (22) and (23)] for the details.

We shall prove Theorem 1.12 later.

## 2. Proofs

### 2.1. Basic properties of binomial coefficients modulo primes

Let us first state a simple fact:

**Proposition 2.1.** Let  $p$  be a prime. Let  $k \in \{1, 2, \dots, p-1\}$ . Then,  $p \mid \binom{p}{k}$ .

Proposition 2.1 is [Grinbe16, Corollary 5.6] and [BenQui03, Theorem 13].

## 2.2. Restating Vandermonde convolution

Let us also derive one more simple corollary of Proposition 1.7:

**Corollary 2.2.** Let  $x \in \mathbb{Z}$  and  $y \in \mathbb{N}$  and  $n \in \mathbb{Z}$ . Then,

$$\binom{x+y}{n} = \sum_{i=0}^y \binom{x}{n-i} \binom{y}{i}. \tag{5}$$

*Proof of Corollary 2.2.* We are in one of the following two cases:

Case 1: We have  $n < 0$ .

Case 2: We have  $n \geq 0$ .

In Case 1, Corollary 2.2 is easy to check, because both sides of (5) are 0 in this case<sup>2</sup>.

Let us now consider Case 2. In this case, we have  $n \geq 0$ . Hence,  $n \in \mathbb{N}$  (since  $n \in \mathbb{Z}$ ).

Define a  $g \in \mathbb{N}$  by  $g = \max\{y, n\}$ . Thus,  $g = \max\{y, n\} \geq y$  and  $g = \max\{y, n\} \geq n$ .

We have  $g \geq y \geq 0$  (since  $y \in \mathbb{N}$ ), so that  $0 \leq y \leq g$ . Hence, we can split the sum  $\sum_{i=0}^g \binom{x}{n-i} \binom{y}{i}$  at  $i = y$ . We thus obtain

$$\begin{aligned} \sum_{i=0}^g \binom{x}{n-i} \binom{y}{i} &= \sum_{i=0}^y \binom{x}{n-i} \binom{y}{i} + \sum_{i=y+1}^g \binom{x}{n-i} \underbrace{\binom{y}{i}}_{=0} \\ &\hspace{15em} \text{(by Proposition 1.3} \\ &\hspace{15em} \text{(since } y < i \text{ (since } i \geq y+1 > y))\text{)}} \\ &= \sum_{i=0}^y \binom{x}{n-i} \binom{y}{i} + \underbrace{\sum_{i=y+1}^g \binom{x}{n-i}}_{=0} 0 \\ &= \sum_{i=0}^y \binom{x}{n-i} \binom{y}{i}. \end{aligned} \tag{6}$$

On the other hand,  $g \geq n \geq 0$ , so that  $0 \leq n \leq g$ . Hence, we can split the sum

---

<sup>2</sup>Indeed, the left-hand side of (5) is 0 (since  $n < 0$ ), and the right-hand side of (5) is 0 (since each  $i \in \{0, 1, \dots, y\}$  satisfies  $n - i \leq n < 0$  and thus  $\binom{x}{n-i} = 0$ ).

---

$\sum_{i=0}^g \binom{x}{n-i} \binom{y}{i}$  at  $i = n$ . We thus obtain

$$\begin{aligned} \sum_{i=0}^g \binom{x}{n-i} \binom{y}{i} &= \sum_{i=0}^n \binom{x}{n-i} \binom{y}{i} + \sum_{i=n+1}^g \underbrace{\binom{x}{n-i}}_{\substack{=0 \\ \text{(since } n-i < 0 \\ \text{(since } i \geq n+1 > n))}} \binom{y}{i} \\ &= \sum_{i=0}^n \binom{x}{n-i} \binom{y}{i} + \underbrace{\sum_{i=n+1}^g 0 \binom{y}{i}}_{=0} \\ &= \sum_{i=0}^n \binom{x}{n-i} \binom{y}{i}. \end{aligned}$$

Comparing this with (6), we find

$$\sum_{i=0}^y \binom{x}{n-i} \binom{y}{i} = \sum_{i=0}^n \binom{x}{n-i} \binom{y}{i}. \tag{7}$$

Proposition 1.7 yields

$$\begin{aligned} \binom{x+y}{n} &= \sum_{k=0}^n \binom{x}{k} \binom{y}{n-k} = \sum_{i=0}^n \binom{x}{n-i} \underbrace{\binom{y}{n-(n-i)}}_{= \binom{y}{i}} \\ &\quad \text{(here, we have substituted } n-i \text{ for } k \text{ in the sum)} \\ &= \sum_{i=0}^n \binom{x}{n-i} \binom{y}{i} = \sum_{i=0}^y \binom{x}{n-i} \binom{y}{i} \end{aligned}$$

(by (7)). This proves Corollary 2.2. □

Let us state a few consequences of Corollary 2.2:

**Corollary 2.3.** Let  $x \in \mathbb{Z}$  and  $n \in \mathbb{Z}$ . Let  $y$  be a positive integer. Then,

$$\binom{x+y}{n} = \binom{x}{n} + \sum_{i=1}^{y-1} \binom{x}{n-i} \binom{y}{i} + \binom{x}{n-y}.$$

*Proof of Corollary 2.3.* We know that  $y$  is a positive integer. Thus, 0 and  $y$  are two

---

distinct elements of  $\{0, 1, \dots, y\}$ . Corollary 2.2 yields

$$\begin{aligned} \binom{x+y}{n} &= \sum_{i=0}^y \binom{x}{n-i} \binom{y}{i} \\ &= \underbrace{\binom{x}{n-0} \binom{y}{0}}_{=1} + \sum_{i=1}^{y-1} \binom{x}{n-i} \binom{y}{i} + \binom{x}{n-y} \underbrace{\binom{y}{y}}_{=1} \\ &\quad \text{(by Proposition 1.4 (applied to } m=y))} \\ &\quad \left( \begin{array}{c} \text{here, we have split off the} \\ \text{addends for } i=0 \text{ and for } i=y \\ \text{from the sum (since 0 and } y \text{ are two} \\ \text{distinct elements of } \{0, 1, \dots, y\}) \end{array} \right) \\ &= \binom{x}{n} + \sum_{i=1}^{y-1} \binom{x}{n-i} \binom{y}{i} + \binom{x}{n-y}. \end{aligned}$$

This proves Corollary 2.3. □

**Corollary 2.4.** Let  $x \in \mathbb{Z}$  and  $n \in \mathbb{Z}$ . Let  $p$  be a prime. Then,

$$\binom{x+p}{n} \equiv \binom{x}{n} + \binom{x}{n-p} \pmod{p}.$$

*Proof of Corollary 2.4.* We have

$$\binom{p}{i} \equiv 0 \pmod{p} \quad \text{for each } i \in \{1, 2, \dots, p-1\} \tag{8}$$

3.

The number  $p$  is a prime, and thus a positive integer. Hence, Corollary 2.3 (applied to  $y = p$ ) yields

$$\begin{aligned} \binom{x+p}{n} &= \binom{x}{n} + \sum_{i=1}^{p-1} \binom{x}{n-i} \underbrace{\binom{p}{i}}_{\substack{\equiv 0 \pmod{p} \\ \text{(by (8))}}} + \binom{x}{n-p} \\ &\equiv \binom{x}{n} + \underbrace{\sum_{i=1}^{p-1} \binom{x}{n-i} 0}_{=0} + \binom{x}{n-p} = \binom{x}{n} + \binom{x}{n-p} \pmod{p}. \end{aligned}$$

This proves Corollary 2.4. □

---

<sup>3</sup>*Proof of (8):* Let  $i \in \{1, 2, \dots, p-1\}$ . Proposition 2.1 (applied to  $k = i$ ) yields  $p \mid \binom{p}{i}$ . In other words,  $\binom{p}{i} \equiv 0 \pmod{p}$ . This proves (8).

### 2.3. The congruence lemma

We now show a general lemma that helps us attack congruences involving binomial coefficients:<sup>4</sup>

**Lemma 2.5.** Let  $A : \mathbb{Z} \times \mathbb{Z} \rightarrow \mathbb{Z}$  be any map. Let  $N$  be an integer. Let  $u \in \mathbb{Z}$ . Assume that the following four conditions hold:

- Every  $a \in \mathbb{Z}$  and  $b \in \mathbb{Z}$  satisfy

$$A(a, b) \equiv A(a-1, b) + A(a-1, b-1) \pmod{N}. \quad (9)$$

- We have

$$A(0, 0) \equiv u \pmod{N}. \quad (10)$$

- Every  $a \in \mathbb{Z}$  and every negative  $b \in \mathbb{Z}$  satisfy

$$A(a, b) \equiv 0 \pmod{N}. \quad (11)$$

- Every positive integer  $b$  satisfies

$$A(0, b) \equiv 0 \pmod{N}. \quad (12)$$

Then, every  $a \in \mathbb{Z}$  and  $b \in \mathbb{Z}$  satisfy

$$A(a, b) \equiv u \binom{a}{b} \pmod{N}.$$

*Proof of Lemma 2.5.* Let us first show the following fact:

*Observation 1:* Let  $b \in \mathbb{Z}$ . We have  $A(0, b) \equiv u \binom{0}{b} \pmod{N}$ .

[*Proof of Observation 1:* We are in one of the following three cases:

*Case 1:* We have  $b < 0$ .

*Case 2:* We have  $b = 0$ .

*Case 3:* We have  $b > 0$ .

Let us first consider Case 1. In this case, we have  $b < 0$ . Thus,  $b$  is a negative integer (since  $b \in \mathbb{Z}$ ). Hence, Definition 1.8 yields  $\binom{0}{b} = 0$ . Thus,  $u \underbrace{\binom{0}{b}}_{=0} = 0$ ,

---

<sup>4</sup>We shall only use Lemma 2.5 in the case when  $N$  is a **positive** integer. For the sake of generality, we are nevertheless stating it for arbitrary integers  $N$ . Make sure to correctly interpret the notation " $u \equiv v \pmod{N}$ " when  $N$  is 0: If  $u$  and  $v$  are two integers, then  $u \equiv v \pmod{0}$  holds if and only if  $u = v$ .

---

so that  $0 = u \binom{0}{b}$ . But (11) (applied to  $a = 0$ ) yields  $A(0, b) \equiv 0 = u \binom{0}{b} \pmod N$ . Thus, Observation 1 is proven in Case 1.

Let us now consider Case 2. In this case, we have  $b = 0$ . Thus,  $u \binom{0}{b} = u \binom{0}{0} = u$ , so that  $u = u \binom{0}{b}$ . But (10) yields  $A(0, 0) \equiv u = u \binom{0}{b} \pmod N$ . From  $b = 0$ , we obtain  $A \left( 0, \underbrace{b}_{=0} \right) = A(0, 0) \equiv u \binom{0}{b} \pmod N$ . Thus, Observation 1 is proven in Case 2.

Finally, let us consider Case 3. In this case, we have  $b > 0$ . Thus,  $b \in \mathbb{N}$  and  $0 < b$ . Hence, Proposition 1.3 (applied to  $m = 0$  and  $n = b$ ) yields  $\binom{0}{b} = 0$ . Hence,  $u \binom{0}{b} = 0$ , so that  $0 = u \binom{0}{b}$ . But (12) yields  $A(0, b) \equiv 0 = u \binom{0}{b} \pmod N$ . Thus, Observation 1 is proven in Case 3.

We have now proven Observation 1 in each of the three Cases 1, 2 and 3. Since these three Cases cover all possibilities, we thus conclude that Observation 1 always holds.]

Next, we claim the following fact:

*Observation 2:* We have  $A(a, b) \equiv u \binom{a}{b} \pmod N$  for each  $a \in \mathbb{N}$  and  $b \in \mathbb{Z}$ .

[*Proof of Observation 2:* We shall prove Observation 2 by induction over  $a$ .

*Induction base:* We have  $A(0, b) \equiv u \binom{0}{b} \pmod N$  for each  $b \in \mathbb{Z}$  (according to Observation 1). In other words, Observation 2 holds for  $a = 0$ . This completes the induction base.

*Induction step:* Let  $c$  be a positive integer. Assume that Observation 2 holds for  $a = c - 1$ . We must prove that Observation 2 holds for  $a = c$ .

We have assumed that Observation 2 holds for  $a = c - 1$ . In other words, we have

$$A(c - 1, b) \equiv u \binom{c - 1}{b} \pmod N \quad \text{for each } b \in \mathbb{Z}. \quad (13)$$

For each  $b \in \mathbb{Z}$ , we have

$$\begin{aligned} \binom{c}{b} &= \binom{c-1}{b-1} + \binom{c-1}{b} \\ &\quad \text{(by Proposition 1.10 (applied to } m = c \text{ and } n = b)) \\ &= \binom{c-1}{b} + \binom{c-1}{b-1}. \end{aligned} \tag{14}$$

Now, for each  $b \in \mathbb{Z}$ , we have

$$\begin{aligned} A(c, b) &\equiv \underbrace{A(c-1, b)}_{\substack{\equiv u \binom{c-1}{b} \pmod{N} \\ \text{(by (13))}}} + \underbrace{A(c-1, b-1)}_{\substack{\equiv u \binom{c-1}{b-1} \pmod{N} \\ \text{(by (13))} \\ \text{(applied to } b-1 \text{ instead of } b)}} \\ &\quad \text{(by (9) (applied to } a = c)) \\ &\equiv u \binom{c-1}{b} + u \binom{c-1}{b-1} = u \underbrace{\left( \binom{c-1}{b} + \binom{c-1}{b-1} \right)}_{\substack{= \binom{c}{b} \\ \text{(by (14))}}} \\ &= u \binom{c}{b} \pmod{N}. \end{aligned}$$

In other words, Observation 2 holds for  $a = c$ . This completes the induction step. Thus, Observation 2 is proven.]

Our next step shall be to prove the following fact:

*Observation 3:* Let  $h \in \mathbb{N}$ . We have  $A(a, b) \equiv u \binom{a}{b} \pmod{N}$  for each  $a \in \mathbb{Z}$  and  $b \in \mathbb{Z}$  satisfying  $b - a < h$ .

[*Proof of Observation 3:* We shall prove Observation 3 by induction over  $h$ :

*Induction base:* We have  $A(a, b) \equiv u \binom{a}{b} \pmod{N}$  for each  $a \in \mathbb{Z}$  and  $b \in \mathbb{Z}$  satisfying  $b - a < 0$ <sup>5</sup>. In other words, Observation 3 holds for  $h = 0$ . This completes the induction base.

---

<sup>5</sup>*Proof.* Let  $a \in \mathbb{Z}$  and  $b \in \mathbb{Z}$  be such that  $b - a < 0$ . We must prove that  $A(a, b) \equiv u \binom{a}{b} \pmod{N}$ .

If  $a \in \mathbb{N}$ , then this follows immediately from Observation 2. Thus, for the rest of this proof, we WLOG assume that we don't have  $a \in \mathbb{N}$ . Hence,  $a \notin \mathbb{N}$ . Combining  $a \in \mathbb{Z}$  with  $a \notin \mathbb{N}$ , we obtain  $a \in \mathbb{Z} \setminus \mathbb{N} = \{-1, -2, -3, \dots\}$ . Hence,  $a < 0$ . But from  $b - a < 0$ , we obtain  $b < a < 0$ . Thus,  $b$  is a negative integer (since  $b \in \mathbb{Z}$ ). Therefore, Definition 1.8 yields  $\binom{a}{b} = 0$ . Hence,

---

*Induction step:* Let  $g \in \mathbb{N}$ . Assume that Observation 3 holds for  $h = g$ . We must prove that Observation 3 holds for  $h = g + 1$ .

We have assumed that Observation 3 holds for  $h = g$ . In other words, we have

$$A(a, b) \equiv u \binom{a}{b} \pmod{N} \quad \text{for each } a \in \mathbb{Z} \text{ and } b \in \mathbb{Z} \\ \text{satisfying } b - a < g. \tag{15}$$

Now, let  $a \in \mathbb{Z}$  and  $b \in \mathbb{Z}$  be such that  $b - a < g + 1$ . Then, (9) (applied to  $a + 1$  instead of  $a$ ) shows that

$$A(a + 1, b) \equiv A \left( \underbrace{(a + 1) - 1}_{=a}, b \right) + A \left( \underbrace{(a + 1) - 1}_{=a}, b - 1 \right) \\ = A(a, b) + A(a, b - 1) \pmod{N}.$$

Hence,

$$A(a, b) \equiv A(a + 1, b) - A(a, b - 1) \pmod{N}. \tag{16}$$

Also, Proposition 1.10 (applied to  $m = a + 1$  and  $n = b$ ) yields

$$\binom{a + 1}{b} = \binom{(a + 1) - 1}{b - 1} + \binom{(a + 1) - 1}{b} = \binom{a}{b - 1} + \binom{a}{b} \\ \text{(since } (a + 1) - 1 = a) \\ = \binom{a}{b} + \binom{a}{b - 1}.$$

Hence,

$$\binom{a}{b} = \binom{a + 1}{b} - \binom{a}{b - 1}. \tag{17}$$

But  $b - (a + 1) = \underbrace{b - a}_{<g+1} - 1 < g + 1 - 1 = g$ . Hence, we can apply (15) to  $a + 1$  instead of  $a$ . We thus obtain

$$A(a + 1, b) \equiv u \binom{a + 1}{b} \pmod{N}.$$

Also,  $(b - 1) - a = \underbrace{b - a}_{<g+1} - 1 < g + 1 - 1 = g$ . Hence, we can apply (15) to  $b - 1$  instead of  $b$ . We thus obtain

$$A(a, b - 1) \equiv u \binom{a}{b - 1} \pmod{N}.$$

---

$u \binom{a}{b} = 0$ , so that  $0 = u \binom{a}{b}$ . But (11) yields  $A(a, b) \equiv 0 = u \binom{a}{b} \pmod{N}$ . Hence, we have  
 $\underbrace{u \binom{a}{b}}_{=0}$   
 proven that  $A(a, b) \equiv u \binom{a}{b} \pmod{N}$ . Qed.

---

Thus, (16) becomes

$$\begin{aligned}
 A(a, b) &\equiv \underbrace{A(a+1, b)} - \underbrace{A(a, b-1)} \\
 &\equiv u \binom{a+1}{b} \pmod{N} \equiv u \binom{a}{b-1} \pmod{N} \\
 &\equiv u \binom{a+1}{b} - u \binom{a}{b-1} = u \underbrace{\left( \binom{a+1}{b} - \binom{a}{b-1} \right)}_{\substack{= \binom{a}{b} \\ \text{(by (17))}}} = u \binom{a}{b} \pmod{N}.
 \end{aligned}$$

Now, forget that we fixed  $a$  and  $b$ . We thus have shown that we have  $A(a, b) \equiv u \binom{a}{b} \pmod{N}$  for each  $a \in \mathbb{Z}$  and  $b \in \mathbb{Z}$  satisfying  $b - a < g + 1$ . In other words, Observation 3 holds for  $h = g + 1$ . This completes the induction step. Thus, Observation 3 is proven.]

Now, let  $a \in \mathbb{Z}$  and  $b \in \mathbb{Z}$  be arbitrary. We must prove that  $A(a, b) \equiv u \binom{a}{b} \pmod{N}$ .

Define  $h \in \mathbb{Z}$  by  $h = \max\{0, b - a + 1\}$ . Thus,  $h = \max\{0, b - a + 1\} \geq 0$ , so that  $h \in \mathbb{N}$  (since  $h \in \mathbb{Z}$ ). Also,  $h = \max\{0, b - a + 1\} \geq b - a + 1 > b - a$ , so that  $b - a < h$ . Hence, Observation 3 shows that we have  $A(a, b) \equiv u \binom{a}{b} \pmod{N}$ . This completes the proof of Lemma 2.5.  $\square$

## 2.4. Proof of the Lucas theorem

We are now ready to prove Theorem 1.11:

*Proof of Theorem 1.11.* Let us forget that we fixed  $a$  and  $b$ .

Define an integer  $u \in \mathbb{Z}$  by  $u = \binom{c}{d}$ . Define a map  $A : \mathbb{Z} \times \mathbb{Z} \rightarrow \mathbb{Z}$  by

$$\left( A(a, b) = \binom{ap + c}{bp + d} \quad \text{for each } (a, b) \in \mathbb{Z} \times \mathbb{Z} \right).$$

Let us now prove some properties of the map  $A$ :

*Observation 1:* Every  $a \in \mathbb{Z}$  and  $b \in \mathbb{Z}$  satisfy

$$A(a, b) \equiv A(a - 1, b) + A(a - 1, b - 1) \pmod{p}.$$

[*Proof of Observation 1:* Let  $a \in \mathbb{Z}$  and  $b \in \mathbb{Z}$ . Then, the definition of  $A$  yields

$$A(a - 1, b) = \binom{(a - 1)p + c}{bp + d}. \tag{18}$$

Also, the definition of  $A$  yields

$$A(a-1, b-1) = \binom{(a-1)p+c}{(b-1)p+d} = \binom{(a-1)p+c}{bp+d-p} \quad (19)$$

(since  $(b-1)p+d = bp+d-p$ ).

Corollary 2.4 (applied to  $x = (a-1)p+c$  and  $n = bp+d$ ) yields

$$\begin{aligned} \binom{(a-1)p+c+p}{bp+d} &\equiv \underbrace{\binom{(a-1)p+c}{bp+d}}_{=A(a-1,b) \text{ (by (18))}} + \underbrace{\binom{(a-1)p+c}{bp+d-p}}_{=A(a-1,b-1) \text{ (by (19))}} \\ &= A(a-1, b) + A(a-1, b-1) \pmod p. \end{aligned} \quad (20)$$

Now, the definition of  $A$  yields

$$\begin{aligned} A(a, b) &= \binom{ap+c}{bp+d} = \binom{(a-1)p+c+p}{bp+d} \quad (\text{since } ap+c = (a-1)p+c+p) \\ &\equiv A(a-1, b) + A(a-1, b-1) \pmod p \end{aligned}$$

(by (20)). This proves Observation 1.]

*Observation 2:* We have  $A(0,0) \equiv u \pmod p$ .

[*Proof of Observation 2:* The definition of  $A$  yields

$$\begin{aligned} A(0,0) &= \binom{0p+c}{0p+d} = \binom{c}{d} \quad (\text{since } 0p+c = c \text{ and } 0p+d = d) \\ &= u \quad \left( \text{since } u = \binom{c}{d} \right) \\ &\equiv u \pmod p. \end{aligned}$$

This proves Observation 2.]

*Observation 3:* Every  $a \in \mathbb{Z}$  and every negative  $b \in \mathbb{Z}$  satisfy

$$A(a, b) \equiv 0 \pmod p.$$

[*Proof of Observation 3:* Let  $a \in \mathbb{Z}$ . Let  $b \in \mathbb{Z}$  be negative. Then,  $bp+d$  is a negative integer<sup>6</sup>. Hence, Definition 1.8 yields  $\binom{ap+c}{bp+d} = 0$ . Now, the definition of  $A$  yields

$$A(a, b) = \binom{ap+c}{bp+d} = 0 \equiv 0 \pmod p.$$

This proves Observation 3.]

---

<sup>6</sup>*Proof.* We have  $d \in \{0, 1, \dots, p-1\}$ , so that  $d \leq p-1 < p$ . But  $b$  is a negative integer (since  $b \in \mathbb{Z}$  is negative); hence,  $b \in \{-1, -2, -3, \dots\}$ , so that  $b \leq -1$ . Hence,  $bp \leq (-1)p$  (since  $p$  is positive). Thus,  $\underbrace{bp}_{\leq (-1)p} + \underbrace{d}_{< p} < (-1)p + p = 0$ . Therefore,  $bp+d$  is a negative integer (since  $bp+d \in \mathbb{Z}$ ). Qed.

Observation 4: Every positive integer  $b$  satisfies

$$A(0, b) \equiv 0 \pmod{p}.$$

[Proof of Observation 4: Let  $b$  be a positive integer. Thus,  $b > 0$ . Also,  $d \in \{0, 1, \dots, p-1\}$ , so that  $d \geq 0$ . Hence,  $\underbrace{b}_{>0} \underbrace{p}_{>0} + \underbrace{d}_{\geq 0} > 0$ . Thus,  $bp + d$  is a

positive integer (since  $bp + d \in \mathbb{Z}$ ), so that  $bp + d \in \mathbb{N}$ . Also,  $c \in \{0, 1, \dots, p-1\} \subseteq \mathbb{N}$ . Moreover,  $b > 0$ , so that  $b \geq 1$  (since  $b$  is an integer). Using  $p > 0$ , we thus find  $\underbrace{b}_{\geq 1} p \geq p$ . But  $c \in \{0, 1, \dots, p-1\}$ , so that  $c \leq p-1 < p$ . Hence,  $p > c$ .

Now,  $bp + \underbrace{d}_{\geq 0} \geq bp \geq p > c$ , so that  $c < bp + d$ . Hence, Proposition 1.3 (applied

to  $m = c$  and  $n = bp + d$ ) yields  $\binom{c}{bp + d} = 0$ .

Now, the definition of  $A$  yields

$$\begin{aligned} A(0, b) &= \binom{0p + c}{bp + d} = \binom{c}{bp + d} \quad (\text{since } 0p + c = c) \\ &= 0 \equiv 0 \pmod{p}. \end{aligned}$$

This proves Observation 4.]

We have now proven the four Observations 1, 2, 3 and 4. In other words, the four conditions in Lemma 2.5 hold if we set  $N = p$ . Thus, Lemma 2.5 (applied to  $N = p$ ) yields that every  $a \in \mathbb{Z}$  and  $b \in \mathbb{Z}$  satisfy

$$A(a, b) \equiv u \binom{a}{b} \pmod{p}. \tag{21}$$

Now, let  $a$  and  $b$  be two integers. Thus,  $a \in \mathbb{Z}$  and  $b \in \mathbb{Z}$ . Hence, (21) yields

$$A(a, b) \equiv \underbrace{u}_{\binom{c}{d}} \binom{a}{b} = \binom{c}{d} \binom{a}{b} = \binom{a}{b} \binom{c}{d} \pmod{p}.$$

In view of

$$A(a, b) = \binom{ap + c}{bp + d} \quad (\text{by the definition of } A),$$

this rewrites as

$$\binom{ap + c}{bp + d} \equiv \binom{a}{b} \binom{c}{d} \pmod{p}.$$

This proves Theorem 1.11. □

## 2.5. Two lemmas for Babbage's theorem

Before we start proving Theorem 1.12, let us show two more auxiliary results. The first one is a consequence of Theorem 1.11:

**Lemma 2.6.** Let  $p$  be a prime. Let  $r \in \mathbb{Z}$  and  $s \in \mathbb{Z}$ . Let  $k \in \{1, 2, \dots, p-1\}$ . Then,  $p \mid \binom{rp}{sp+k}$ .

*Proof of Lemma 2.6.* From  $k \in \{1, 2, \dots, p-1\}$ , we conclude that  $k$  is a positive integer. Thus,  $k > 0$ . Hence,  $0 < k$ . Also,  $k \in \{1, 2, \dots, p-1\} \subseteq \mathbb{N}$ . Thus, Proposition 1.3 (applied to  $m = 0$  and  $n = k$ ) yields  $\binom{0}{k} = 0$ .

We have  $k \in \{1, 2, \dots, p-1\} \subseteq \{0, 1, \dots, p-1\}$ . Also,  $0 \in \{0, 1, \dots, p-1\}$  (since  $p-1 \in \mathbb{N}$  (since  $p$  is a positive integer)). Thus, Theorem 1.11 (applied to  $a = r$ ,  $b = s$ ,  $c = 0$  and  $d = k$ ) yields

$$\binom{rp+0}{sp+k} \equiv \binom{r}{s} \underbrace{\binom{0}{k}}_{=0} = 0 \pmod{p}.$$

In other words,  $p \mid \binom{rp+0}{sp+k}$ . In view of  $rp+0 = rp$ , this rewrites as  $p \mid \binom{rp}{sp+k}$ . Hence, Lemma 2.6 is proven.  $\square$

The next auxiliary result is similar to Corollary 2.4, and also follows from Corollary 2.3:

**Corollary 2.7.** Let  $r \in \mathbb{Z}$  and  $b \in \mathbb{Z}$ . Let  $p$  be a prime. Then,

$$\binom{(r+1)p}{bp} \equiv \binom{rp}{bp} + \binom{rp}{(b-1)p} \pmod{p^2}.$$

*Proof of Corollary 2.7.* We have

$$\binom{rp}{bp-i} \binom{p}{i} \equiv 0 \pmod{p^2} \quad \text{for each } i \in \{1, 2, \dots, p-1\} \quad (22)$$

7.

---

<sup>7</sup>Proof of (22): Let  $i \in \{1, 2, \dots, p-1\}$ . Proposition 2.1 (applied to  $k = i$ ) yields  $p \mid \binom{p}{i}$ . In other

words, there exists an  $x \in \mathbb{Z}$  such that  $\binom{p}{i} = px$ . Consider this  $x$ .

On the other hand, from  $i \in \{1, 2, \dots, p-1\}$ , we obtain  $p-i \in \{1, 2, \dots, p-1\}$ . Hence,

---

The number  $p$  is a prime, and thus a positive integer. Hence, Corollary 2.3 (applied to  $x = rp$ ,  $y = p$  and  $n = bp$ ) yields

$$\begin{aligned} \binom{rp+p}{bp} &= \binom{rp}{bp} + \sum_{i=1}^{p-1} \underbrace{\binom{rp}{bp-i} \binom{p}{i}}_{\substack{\equiv 0 \pmod{p^2} \\ \text{(by (22))}}} + \underbrace{\binom{rp}{bp-p}}_{\substack{= \binom{rp}{(b-1)p} \\ \text{(since } bp-p=(b-1)p)}} \\ &\equiv \binom{rp}{bp} + \underbrace{\sum_{i=1}^{p-1} 0}_{=0} + \binom{rp}{(b-1)p} = \binom{rp}{bp} + \binom{rp}{(b-1)p} \pmod{p^2}. \end{aligned}$$

In view of  $rp + p = (r + 1)p$ , this rewrites as

$$\binom{(r+1)p}{bp} \equiv \binom{rp}{bp} + \binom{rp}{(b-1)p} \pmod{p^2}.$$

This proves Corollary 2.7. □

## 2.6. Proof of Babbage's theorem

We are now ready to prove Theorem 1.12:

*Proof of Theorem 1.12.* Let us forget that we fixed  $a$  and  $b$ .

Define an integer  $u \in \mathbb{Z}$  by  $u = 1$ . Define a map  $A : \mathbb{Z} \times \mathbb{Z} \rightarrow \mathbb{Z}$  by

$$\left( A(a, b) = \binom{ap}{bp} \quad \text{for each } (a, b) \in \mathbb{Z} \times \mathbb{Z} \right).$$

Let us now prove some properties of the map  $A$ :

*Observation 1:* Every  $a \in \mathbb{Z}$  and  $b \in \mathbb{Z}$  satisfy

$$A(a, b) \equiv A(a-1, b) + A(a-1, b-1) \pmod{p^2}.$$

Lemma 2.6 (applied to  $s = b - 1$  and  $k = p - i$ ) yields  $p \mid \binom{rp}{(b-1)p+p-i} = \binom{rp}{bp-i}$  (since  $(b-1)p + p - i = bp - i$ ). In other words, there exists a  $y \in \mathbb{Z}$  such that  $\binom{rp}{bp-i} = py$ . Consider this  $y$ .

We have

$$\underbrace{\binom{rp}{bp-i}}_{=py} \underbrace{\binom{p}{i}}_{=px} = pypx = p^2xy \equiv 0 \pmod{p^2}.$$

This proves (22).

[Proof of Observation 1: Let  $a \in \mathbb{Z}$  and  $b \in \mathbb{Z}$ . Then, the definition of  $A$  yields

$$A(a-1, b) = \binom{(a-1)p}{bp}. \quad (23)$$

Also, the definition of  $A$  yields

$$A(a-1, b-1) = \binom{(a-1)p}{(b-1)p}. \quad (24)$$

Corollary 2.7 (applied to  $r = a - 1$ ) yields

$$\begin{aligned} \binom{((a-1)+1)p}{bp} &\equiv \underbrace{\binom{(a-1)p}{bp}}_{=A(a-1,b) \text{ (by (23))}} + \underbrace{\binom{(a-1)p}{(b-1)p}}_{=A(a-1,b-1) \text{ (by (24))}} \\ &= A(a-1, b) + A(a-1, b-1) \pmod{p^2}. \end{aligned} \quad (25)$$

Now, the definition of  $A$  yields

$$\begin{aligned} A(a, b) &= \binom{ap}{bp} = \binom{((a-1)+1)p}{bp} \quad (\text{since } a = (a-1) + 1) \\ &\equiv A(a-1, b) + A(a-1, b-1) \pmod{p^2} \end{aligned}$$

(by (25)). This proves Observation 1.]

*Observation 2:* We have  $A(0, 0) \equiv u \pmod{p^2}$ .

[Proof of Observation 2: The definition of  $A$  yields

$$A(0, 0) = \binom{0p}{0p} = \binom{0}{0} = 1 = u \equiv u \pmod{p^2}.$$

This proves Observation 2.]

*Observation 3:* Every  $a \in \mathbb{Z}$  and every negative  $b \in \mathbb{Z}$  satisfy

$$A(a, b) \equiv 0 \pmod{p^2}.$$

[Proof of Observation 3: Let  $a \in \mathbb{Z}$ . Let  $b \in \mathbb{Z}$  be negative. Then,  $bp$  is a negative integer (since  $b$  is negative but  $p$  is positive). Hence, Definition 1.8 yields  $\binom{ap}{bp} = 0$ .

Now, the definition of  $A$  yields

$$A(a, b) = \binom{ap}{bp} = 0 \equiv 0 \pmod{p^2}.$$

This proves Observation 3.]

---

*Observation 4:* Every positive integer  $b$  satisfies

$$A(0, b) \equiv 0 \pmod{p^2}.$$

[*Proof of Observation 4:* Let  $b$  be a positive integer. Thus,  $b > 0$ . Hence,  $bp > 0$  (since  $p$  is positive). Thus,  $bp$  is a positive integer (since  $bp \in \mathbb{Z}$ ), so that  $bp \in \mathbb{N}$ . Moreover,  $0 < bp$  (since  $bp > 0$ ). Hence, Proposition 1.3 (applied to  $m = 0$  and  $n = bp$ ) yields  $\binom{0}{bp} = 0$ .

Now, the definition of  $A$  yields

$$\begin{aligned} A(0, b) &= \binom{0p}{bp} = \binom{0}{bp} && (\text{since } 0p = 0) \\ &= 0 \equiv 0 \pmod{p^2}. \end{aligned}$$

This proves Observation 4.]

We have now proven the four Observations 1, 2, 3 and 4. In other words, the four conditions in Lemma 2.5 hold if we set  $N = p^2$ . Thus, Lemma 2.5 (applied to  $N = p^2$ ) yields that every  $a \in \mathbb{Z}$  and  $b \in \mathbb{Z}$  satisfy

$$A(a, b) \equiv u \binom{a}{b} \pmod{p^2}. \quad (26)$$

Now, let  $a$  and  $b$  be two integers. Thus,  $a \in \mathbb{Z}$  and  $b \in \mathbb{Z}$ . Hence, (26) yields

$$A(a, b) \equiv \underbrace{u}_{=1} \binom{a}{b} = \binom{a}{b} \pmod{p^2}.$$

In view of

$$A(a, b) = \binom{ap}{bp} \quad (\text{by the definition of } A),$$

this rewrites as

$$\binom{ap}{bp} \equiv \binom{a}{b} \pmod{p^2}.$$

This proves Theorem 1.12. □

### 3. The sums of the first $p$ powers

#### 3.1. The congruence

Next, we shall prove a well-known congruence concerning the sum  $\sum_{l=0}^{p-1} l^k = 0^k + 1^k + \cdots + (p-1)^k$  for a prime  $p$ :

---

**Theorem 3.1.** Let  $p$  be a prime. Let  $k \in \mathbb{N}$ . Assume that  $k$  is not a positive multiple of  $p - 1$ . Then,

$$\sum_{l=0}^{p-1} l^k \equiv 0 \pmod{p}.$$

Theorem 3.1 has nothing to do with binomial coefficients. Nevertheless, we shall prove it using binomial coefficients.

### 3.2. Powers and power sums via Stirling numbers of the second kind

We shall first introduce another family of integers: the so-called *Stirling numbers of the second kind*. They have various equivalent definitions; we define them by recursion:

**Definition 3.2.** For each  $m \in \mathbb{N}$  and  $n \in \mathbb{Z}$ , we define an integer  $\left\{ \begin{matrix} m \\ n \end{matrix} \right\}$  as follows:

We proceed by recursion on  $m$ :

- We set

$$\left\{ \begin{matrix} 0 \\ n \end{matrix} \right\} = \begin{cases} 1, & \text{if } n = 0; \\ 0, & \text{if } n \neq 0 \end{cases} \quad \text{for all } n \in \mathbb{Z}. \quad (27)$$

This defines  $\left\{ \begin{matrix} m \\ n \end{matrix} \right\}$  for  $m = 0$ .

- For each positive integer  $m$  and each  $n \in \mathbb{Z}$ , we set

$$\left\{ \begin{matrix} m \\ n \end{matrix} \right\} = n \left\{ \begin{matrix} m-1 \\ n \end{matrix} \right\} + \left\{ \begin{matrix} m-1 \\ n-1 \end{matrix} \right\}. \quad (28)$$

Thus, a family  $\left( \left\{ \begin{matrix} m \\ n \end{matrix} \right\} \right)_{(m,n) \in \mathbb{N} \times \mathbb{Z}}$  of integers is defined. These integers  $\left\{ \begin{matrix} m \\ n \end{matrix} \right\}$  are called the *Stirling numbers of the second kind*.

These Stirling numbers  $\left\{ \begin{matrix} m \\ n \end{matrix} \right\}$  have a well-known combinatorial interpretation:

Namely, if  $m \in \mathbb{N}$  and  $n \in \mathbb{N}$ , then  $\left\{ \begin{matrix} m \\ n \end{matrix} \right\}$  is the number of set partitions of the set  $\{1, 2, \dots, m\}$  into  $n$  nonempty subsets. This is actually not hard to prove by induction on  $m$  (for example, the proof is sketched in [Stan11, §1.9] and in [GrKnPa, §6.1]<sup>8</sup>); but we don't need this. Instead, let us prove the following algebraic facts:

---

<sup>8</sup>To be more precise, both [Stan11, §1.9] and [GrKnPa, §6.1] **define**  $\left\{ \begin{matrix} m \\ n \end{matrix} \right\}$  as the number of set

**Proposition 3.3.** For each  $m \in \mathbb{N}$  and  $n \in \mathbb{Z}$  satisfying  $n \notin \{0, 1, \dots, m\}$ , we have

$$\left\{ \begin{matrix} m \\ n \end{matrix} \right\} = 0.$$

*Proof of Proposition 3.3.* We shall prove Proposition 3.3 by induction on  $m$ :

*Induction base:* Proposition 3.3 holds when  $m = 0$  (as follows easily from (27)).

This completes the induction base.

*Induction step:* Let  $k$  be a positive integer. Assume that Proposition 3.3 holds when  $m = k - 1$ . We must now prove that Proposition 3.3 holds when  $m = k$ .

We have assumed that Proposition 3.3 holds when  $m = k - 1$ . In other words, for each  $n \in \mathbb{Z}$  satisfying  $n \notin \{0, 1, \dots, k - 1\}$ , we have

$$\left\{ \begin{matrix} k - 1 \\ n \end{matrix} \right\} = 0. \quad (29)$$

Now, let  $n \in \mathbb{Z}$  be such that  $n \notin \{0, 1, \dots, k\}$ . Thus,  $n - 1 \notin \{0, 1, \dots, k - 1\}$ .

Hence, (29) (applied to  $n - 1$  instead of  $n$ ) yields  $\left\{ \begin{matrix} k - 1 \\ n - 1 \end{matrix} \right\} = 0$ . Also,  $n \notin \{0, 1, \dots, k - 1\}$

(this again follows from  $n \notin \{0, 1, \dots, k\}$ ). Hence, (29) yields  $\left\{ \begin{matrix} k - 1 \\ n \end{matrix} \right\} = 0$ . Now,

(28) (applied to  $m = k$ ) yields

$$\left\{ \begin{matrix} k \\ n \end{matrix} \right\} = n \underbrace{\left\{ \begin{matrix} k - 1 \\ n \end{matrix} \right\}}_{=0} + \underbrace{\left\{ \begin{matrix} k - 1 \\ n - 1 \end{matrix} \right\}}_{=0} = 0.$$

Now, forget that we fixed  $n$ . We thus have shown that for each  $n \in \mathbb{Z}$  satisfying  $n \notin \{0, 1, \dots, k\}$ , we have  $\left\{ \begin{matrix} k \\ n \end{matrix} \right\} = 0$ . In other words, Proposition 3.3 holds when  $m = k$ . This completes the induction step. Thus, the proof of Proposition 3.3 is complete.  $\square$

**Lemma 3.4.** Let  $j \in \mathbb{N}$  and  $x \in \mathbb{Q}$ . Then,

$$j! (x - j) \binom{x}{j} = (j + 1)! \binom{x}{j + 1}.$$

*Proof of Lemma 3.4.* We have  $j \in \mathbb{N}$ . Thus, the definition of  $\binom{x}{j}$  yields

$$\binom{x}{j} = \frac{x(x - 1) \cdots (x - j + 1)}{j!}.$$

---

partitions of the set  $\{1, 2, \dots, m\}$  into  $n$  nonempty subsets, and then prove that (27) and (28) hold with this definition. This is exactly the opposite of what we are doing; but of course, it is equivalent.

---

Hence,

$$\begin{aligned}
 j!(x-j) \binom{x}{j} &= j!(x-j) \cdot \frac{x(x-1)\cdots(x-j+1)}{j!} \\
 &= \frac{x(x-1)\cdots(x-j+1)}{j!} \\
 &= (x-j) \cdot (x(x-1)\cdots(x-j+1)) \\
 &= (x(x-1)\cdots(x-j+1)) \cdot (x-j) \\
 &= x(x-1)\cdots(x-j). \tag{30}
 \end{aligned}$$

On the other hand,  $j+1 \in \mathbb{N}$  (since  $j \in \mathbb{N}$ ). Hence, the definition of  $\binom{x}{j+1}$  yields

$$\binom{x}{j+1} = \frac{x(x-1)\cdots(x-(j+1)+1)}{(j+1)!}.$$

Hence,

$$\begin{aligned}
 (j+1)! \binom{x}{j+1} &= x(x-1)\cdots(x-(j+1)+1) \\
 &= x(x-1)\cdots(x-j) \quad (\text{since } x-(j+1)+1 = x-j) \\
 &= j!(x-j) \binom{x}{j} \quad (\text{by (30)}).
 \end{aligned}$$

This proves Lemma 3.4. □

**Proposition 3.5.** Let  $m \in \mathbb{N}$  and  $x \in \mathbb{Q}$ . Then,

$$x^m = \sum_{j=0}^m j! \left\{ \begin{matrix} m \\ j \end{matrix} \right\} \binom{x}{j}.$$

*Proof of Proposition 3.5.* We shall prove Proposition 3.5 by induction on  $m$ :

*Induction base:* It is straightforward to see that Proposition 3.5 holds when  $m = 0$ . This completes the induction base.

*Induction step:* Let  $k$  be a positive integer. Assume that Proposition 3.5 holds when  $m = k - 1$ . We must now prove that Proposition 3.5 holds when  $m = k$ .

We have assumed that Proposition 3.5 holds when  $m = k - 1$ . In other words, we have

$$x^{k-1} = \sum_{j=0}^{k-1} j! \left\{ \begin{matrix} k-1 \\ j \end{matrix} \right\} \binom{x}{j}.$$


---

Multiplying both sides of this equality by  $x$ , we obtain

$$\begin{aligned}
 x^{k-1}x &= \left( \sum_{j=0}^{k-1} j! \left\{ \begin{matrix} k-1 \\ j \end{matrix} \right\} \binom{x}{j} \right) x = \sum_{j=0}^{k-1} j! \left\{ \begin{matrix} k-1 \\ j \end{matrix} \right\} \binom{x}{j} \underbrace{x}_{=j+(x-j)} \\
 &= \sum_{j=0}^{k-1} \underbrace{j! \left\{ \begin{matrix} k-1 \\ j \end{matrix} \right\} \binom{x}{j}}_{=j! \left\{ \begin{matrix} k-1 \\ j \end{matrix} \right\} \binom{x}{j} j + j! \left\{ \begin{matrix} k-1 \\ j \end{matrix} \right\} \binom{x}{j} (x-j)} (j + (x - j)) \\
 &= \sum_{j=0}^{k-1} \left( j! \left\{ \begin{matrix} k-1 \\ j \end{matrix} \right\} \binom{x}{j} j + j! \left\{ \begin{matrix} k-1 \\ j \end{matrix} \right\} \binom{x}{j} (x - j) \right) \\
 &= \sum_{j=0}^{k-1} j! \left\{ \begin{matrix} k-1 \\ j \end{matrix} \right\} \binom{x}{j} j + \sum_{j=0}^{k-1} j! \left\{ \begin{matrix} k-1 \\ j \end{matrix} \right\} \binom{x}{j} (x - j). \tag{31}
 \end{aligned}$$

But Proposition 3.3 (applied to  $m = k - 1$  and  $n = k$ ) yields  $\left\{ \begin{matrix} k-1 \\ k \end{matrix} \right\} = 0$ , whereas Proposition 3.3 (applied to  $m = k - 1$  and  $n = -1$ ) yields  $\left\{ \begin{matrix} k-1 \\ -1 \end{matrix} \right\} = 0$ .

But (28) (applied to  $m = k$  and  $n = j$ ) yields

$$\left\{ \begin{matrix} k \\ j \end{matrix} \right\} = j \left\{ \begin{matrix} k-1 \\ j \end{matrix} \right\} + \left\{ \begin{matrix} k-1 \\ j-1 \end{matrix} \right\}. \tag{32}$$

We have  $k \in \mathbb{N}$  (since  $k$  is a positive integer), so that  $k \in \{0, 1, \dots, k\}$ . Now,

$$\begin{aligned}
 &\sum_{j=0}^k j! \left\{ \begin{matrix} k-1 \\ j \end{matrix} \right\} \binom{x}{j} j \\
 &= \sum_{j=0}^{k-1} j! \left\{ \begin{matrix} k-1 \\ j \end{matrix} \right\} \binom{x}{j} j + \underbrace{k! \left\{ \begin{matrix} k-1 \\ k \end{matrix} \right\} \binom{x}{k} k}_{=0} \\
 &\quad \left( \begin{array}{l} \text{here, we have split off the addend for } j = k \text{ from the sum} \\ \text{(since } k \in \{0, 1, \dots, k\}) \end{array} \right) \\
 &= \sum_{j=0}^{k-1} j! \left\{ \begin{matrix} k-1 \\ j \end{matrix} \right\} \binom{x}{j} j + \underbrace{k! 0 \binom{x}{k} k}_{=0} = \sum_{j=0}^{k-1} j! \left\{ \begin{matrix} k-1 \\ j \end{matrix} \right\} \binom{x}{j} j,
 \end{aligned}$$

so that

$$\sum_{j=0}^{k-1} j! \left\{ \begin{matrix} k-1 \\ j \end{matrix} \right\} \binom{x}{j} j = \sum_{j=0}^k j! \left\{ \begin{matrix} k-1 \\ j \end{matrix} \right\} \binom{x}{j} j. \tag{33}$$

Also,  $0 \in \{0, 1, \dots, k\}$  (since  $k \in \mathbb{N}$ ). Now,

$$\begin{aligned}
 & \sum_{j=0}^{k-1} j! \underbrace{\left\{ \begin{matrix} k-1 \\ j \end{matrix} \right\} \binom{x}{j}}_{= \binom{x}{j} \left\{ \begin{matrix} k-1 \\ j \end{matrix} \right\}} (x-j) \\
 &= \sum_{j=0}^{k-1} j! (x-j) \binom{x}{j} \left\{ \begin{matrix} k-1 \\ j \end{matrix} \right\} \\
 &= \sum_{j=0}^{k-1} (j+1)! \binom{x}{j+1} \left\{ \begin{matrix} k-1 \\ (j+1)-1 \end{matrix} \right\} \\
 & \quad \text{(by Lemma 3.4) (since } j=(j+1)-1 \text{)} \\
 &= \sum_{j=0}^{k-1} (j+1)! \binom{x}{j+1} \left\{ \begin{matrix} k-1 \\ (j+1)-1 \end{matrix} \right\} \\
 &= \sum_{j=1}^k j! \binom{x}{j} \left\{ \begin{matrix} k-1 \\ j-1 \end{matrix} \right\} \\
 & \quad \text{(here, we have substituted } j \text{ for } j+1 \text{ in the sum).}
 \end{aligned}$$

Comparing this with

$$\begin{aligned}
 & \sum_{j=0}^k j! \binom{x}{j} \left\{ \begin{matrix} k-1 \\ j-1 \end{matrix} \right\} \\
 &= \sum_{j=1}^k j! \binom{x}{j} \left\{ \begin{matrix} k-1 \\ j-1 \end{matrix} \right\} + 0! \binom{x}{0} \underbrace{\left\{ \begin{matrix} k-1 \\ 0-1 \end{matrix} \right\}}_{= \left\{ \begin{matrix} k-1 \\ -1 \end{matrix} \right\} = 0} \\
 & \quad \left( \text{here, we have split off the addend for } j=0 \text{ from the sum} \right) \\
 & \quad \quad \quad \text{(since } 0 \in \{0, 1, \dots, k\} \text{)} \\
 &= \sum_{j=1}^k j! \binom{x}{j} \left\{ \begin{matrix} k-1 \\ j-1 \end{matrix} \right\} + \underbrace{0! \binom{x}{0}}_{=0} 0 = \sum_{j=1}^k j! \binom{x}{j} \left\{ \begin{matrix} k-1 \\ j-1 \end{matrix} \right\},
 \end{aligned}$$

we find

$$\sum_{j=0}^{k-1} j! \left\{ \begin{matrix} k-1 \\ j \end{matrix} \right\} \binom{x}{j} (x-j) = \sum_{j=0}^k j! \binom{x}{j} \left\{ \begin{matrix} k-1 \\ j-1 \end{matrix} \right\}. \tag{34}$$

Comparing the equality (31) with  $x^{k-1}x = x^k$ , we find

$$\begin{aligned}
 x^k &= \underbrace{\sum_{j=0}^{k-1} j! \left\{ \begin{matrix} k-1 \\ j \end{matrix} \right\} \binom{x}{j}}_j + \underbrace{\sum_{j=0}^{k-1} j! \left\{ \begin{matrix} k-1 \\ j \end{matrix} \right\} \binom{x}{j}}_{(x-j)} \\
 &= \sum_{j=0}^k j! \left\{ \begin{matrix} k-1 \\ j \end{matrix} \right\} \binom{x}{j} \quad \quad \quad = \sum_{j=0}^k j! \binom{x}{j} \left\{ \begin{matrix} k-1 \\ j-1 \end{matrix} \right\} \\
 &\quad \quad \quad \text{(by (33))} \quad \quad \quad \text{(by (34))} \\
 &= \sum_{j=0}^k j! \left\{ \begin{matrix} k-1 \\ j \end{matrix} \right\} \binom{x}{j} + \sum_{j=0}^k j! \binom{x}{j} \left\{ \begin{matrix} k-1 \\ j-1 \end{matrix} \right\} \\
 &= \sum_{j=0}^k \underbrace{\left( j! \left\{ \begin{matrix} k-1 \\ j \end{matrix} \right\} \binom{x}{j} + j! \binom{x}{j} \left\{ \begin{matrix} k-1 \\ j-1 \end{matrix} \right\} \right)}_{=j! \left( j \left\{ \begin{matrix} k-1 \\ j \end{matrix} \right\} + \left\{ \begin{matrix} k-1 \\ j-1 \end{matrix} \right\} \right) \binom{x}{j}} \\
 &= \sum_{j=0}^k j! \underbrace{\left( j \left\{ \begin{matrix} k-1 \\ j \end{matrix} \right\} + \left\{ \begin{matrix} k-1 \\ j-1 \end{matrix} \right\} \right)}_{= \left\{ \begin{matrix} k \\ j \end{matrix} \right\} \text{ (by (32))}} \binom{x}{j} = \sum_{j=0}^k j! \left\{ \begin{matrix} k \\ j \end{matrix} \right\} \binom{x}{j}.
 \end{aligned}$$

In other words, Proposition 3.5 holds when  $m = k$ . This completes the induction step. Thus, Proposition 3.5 is proven. □

Next, we shall prove another basic identity about binomial coefficients, sometimes known as the *hockey-stick identity* (in this or another equivalent form):

**Proposition 3.6.** Let  $j \in \mathbb{N}$  and  $h \in \mathbb{N}$ . Then,

$$\sum_{x=0}^h \binom{x}{j} = \binom{h+1}{j+1}.$$

*Proof of Proposition 3.6.* For each  $x \in \mathbb{N}$ , we have

$$\binom{x}{j} = \binom{x+1}{j+1} - \binom{x}{j+1} \tag{35}$$

9.

---

<sup>9</sup>Proof of (35): Let  $x \in \mathbb{N}$ . Then, Proposition 1.10 (applied to  $m = x + 1$  and  $n = j + 1$ ) yields

$$\binom{x+1}{j+1} = \binom{(x+1)-1}{(j+1)-1} + \binom{(x+1)-1}{j+1} = \binom{x}{j} + \binom{x}{j+1}$$

Proposition 1.3 (applied to  $m = 0$  and  $n = j + 1$ ) yields  $\binom{0}{j+1} = 0$  (since  $0 \leq j < j + 1$ ).

But

$$\begin{aligned} \sum_{x=0}^{h+1} \binom{x}{j+1} &= \sum_{x=1}^{h+1} \binom{x}{j+1} + \underbrace{\binom{0}{j+1}}_{=0} \\ &\quad \left( \begin{array}{l} \text{here, we have split off the addend for } x = 0 \text{ from the sum} \\ \text{(since } 0 \in \{0, 1, \dots, h + 1\}) \end{array} \right) \\ &= \sum_{x=1}^{h+1} \binom{x}{j+1} = \sum_{x=0}^h \binom{x+1}{j+1} \end{aligned}$$

(here, we have substituted  $x + 1$  for  $x$  in the sum). Hence,

$$\begin{aligned} \sum_{x=0}^h \binom{x+1}{j+1} &= \sum_{x=0}^{h+1} \binom{x}{j+1} = \sum_{x=0}^h \binom{x}{j+1} + \binom{h+1}{j+1} \tag{36} \\ &\quad \left( \begin{array}{l} \text{here, we have split off the addend for } x = h + 1 \text{ from the sum} \\ \text{(since } h + 1 \in \{0, 1, \dots, h + 1\} \text{ (since } h + 1 \in \mathbb{N}) \end{array} \right). \end{aligned}$$

Now,

$$\begin{aligned} \sum_{x=0}^h \binom{x}{j} &= \underbrace{\binom{x}{j}}_{\substack{= \binom{x+1}{j+1} - \binom{x}{j+1} \\ \text{(by (35))}}} \\ &= \sum_{x=0}^h \left( \binom{x+1}{j+1} - \binom{x}{j+1} \right) = \underbrace{\sum_{x=0}^h \binom{x+1}{j+1}}_{\substack{= \sum_{x=0}^h \binom{x}{j+1} + \binom{h+1}{j+1} \\ \text{(by (36))}}} - \sum_{x=0}^h \binom{x}{j+1} \\ &= \sum_{x=0}^h \binom{x}{j+1} + \binom{h+1}{j+1} - \sum_{x=0}^h \binom{x}{j+1} = \binom{h+1}{j+1}. \end{aligned}$$

This proves Proposition 3.6. □

We can now obtain a reasonably simple formula for sums of the form  $\sum_{x=0}^h x^m$ :

---

(since  $(x + 1) - 1 = x$  and  $(j + 1) - 1 = j$ ). Solving this equation for  $\binom{x}{j}$ , we obtain  $\binom{x}{j} = \binom{x+1}{j+1} - \binom{x}{j+1}$ . This proves (35).

---

**Theorem 3.7.** Let  $m \in \mathbb{N}$  and  $h \in \mathbb{N}$ . Then,

$$\sum_{x=0}^h x^m = \sum_{j=0}^m j! \left\{ \begin{matrix} m \\ j \end{matrix} \right\} \binom{h+1}{j+1}.$$

*Proof of Theorem 3.7.* We have

$$\begin{aligned} \sum_{x=0}^h x^m &= \sum_{j=0}^m j! \left\{ \begin{matrix} m \\ j \end{matrix} \right\} \binom{h+1}{j+1} \\ &= \sum_{j=0}^m j! \left\{ \begin{matrix} m \\ j \end{matrix} \right\} \binom{x}{j} \Big|_{x=0}^h \\ &= \sum_{j=0}^m \sum_{x=0}^h j! \left\{ \begin{matrix} m \\ j \end{matrix} \right\} \binom{x}{j} \\ &= \sum_{j=0}^m j! \left\{ \begin{matrix} m \\ j \end{matrix} \right\} \underbrace{\sum_{x=0}^h \binom{x}{j}}_{\binom{h+1}{j+1}} \\ &= \sum_{j=0}^m j! \left\{ \begin{matrix} m \\ j \end{matrix} \right\} \binom{h+1}{j+1}. \end{aligned}$$

(by Proposition 3.6)

This proves Theorem 3.7. □

We are now ready to prove the following particular case of Theorem 3.1:

**Lemma 3.8.** Let  $p$  be a prime. Let  $k \in \mathbb{N}$ . Assume that  $k < p - 1$ . Then,

$$\sum_{l=0}^{p-1} l^k \equiv 0 \pmod{p}.$$

*Proof of Lemma 3.8.* We have  $k < p - 1$ , so that  $k + 1 < p$ . Since  $k + 1$  and  $p$  are integers, this yields  $k + 1 \leq p - 1$ .

For each  $j \in \{0, 1, \dots, k\}$ , we have

$$\binom{p}{j+1} \equiv 0 \pmod{p} \tag{37}$$

10.

---

<sup>10</sup>*Proof of (37):* Let  $j \in \{0, 1, \dots, k\}$ . Thus,  $0 \leq j \leq k$ . From  $j \geq 0$ , we obtain  $\underbrace{j}_{\geq 0} + 1 \geq 1$ . Combining

this with  $\underbrace{j}_{\leq k} + 1 \leq k + 1 \leq p - 1$ , we obtain  $1 \leq j + 1 \leq p - 1$ . Hence,  $j + 1 \in \{1, 2, \dots, p - 1\}$ .

Thus, Proposition 2.1 (applied to  $j + 1$  instead of  $k$ ) yields  $p \mid \binom{p}{j+1}$ . In other words,  $\binom{p}{j+1} \equiv 0 \pmod{p}$ . This proves (37).

Now,  $p - 1 \in \mathbb{N}$  (since  $p \geq 1$  (since  $p$  is a prime)). Thus, Theorem 3.7 (applied to  $h = p - 1$  and  $m = k$ ) yields

$$\begin{aligned} \sum_{x=0}^{p-1} x^k &= \sum_{j=0}^k j! \binom{k}{j} \binom{(p-1)+1}{j+1} = \sum_{j=0}^k j! \binom{k}{j} \underbrace{\binom{p}{j+1}}_{\substack{\equiv 0 \pmod p \\ \text{(by (37))}}} \quad (\text{since } (p-1)+1 = p) \\ &\equiv \sum_{j=0}^k j! \binom{k}{j} 0 = 0 \pmod p. \end{aligned}$$

Now,

$$\begin{aligned} \sum_{l=0}^{p-1} l^k &= \sum_{x=0}^{p-1} x^k \quad (\text{here, we have renamed the summation index } l \text{ as } x) \\ &\equiv 0 \pmod p. \end{aligned}$$

This proves Lemma 3.8. □

### 3.3. Finishing the proof

The last ingredient we need for the proof of Theorem 3.1 is *Fermat's little theorem*:

**Proposition 3.9.** Let  $p$  be a prime. Let  $a \in \mathbb{Z}$ . Then,  $a^p \equiv a \pmod p$ .

Proposition 3.9 is, of course, one of the fundamental facts of number theory, and shall not be proven here. We shall use the following corollary of Proposition 3.9:

**Corollary 3.10.** Let  $p$  be a prime. Let  $a \in \mathbb{Z}$ . Let  $k$  be a positive integer. Let  $r$  be the remainder of  $k$  upon division by  $p - 1$ . Assume that  $k$  is not a multiple of  $p - 1$ . Then,  $a^k \equiv a^r \pmod p$ .

*Proof of Corollary 3.10.* The definition of  $r$  shows that  $r \in \{0, 1, \dots, (p - 1) - 1\}$  and  $r \equiv k \pmod{p - 1}$  and  $r \leq k$  (since  $k \geq 0$ ). But  $k \not\equiv 0 \pmod{p - 1}$  (since  $k$  is not a multiple of  $p - 1$ ). Hence,  $r \equiv k \not\equiv 0 \pmod{p - 1}$ , so that  $r \neq 0$ .

From  $k \equiv r \pmod{p - 1}$ , we obtain  $p - 1 \mid k - r$ . Thus, there exists a  $q \in \mathbb{Z}$  such that  $k - r = (p - 1)q$ . Consider this  $q$ . We have  $(p - 1)q = k - r \geq 0$  (since  $r \leq k$ ) and thus  $q \geq 0$  (since  $p - 1 > 0$ ). In other words,  $q \in \mathbb{N}$ .

Proposition 3.9 yields  $a^p \equiv a \pmod p$ . Hence,

$$a^{(p-1)m} \equiv a \pmod p \quad \text{for each } m \in \mathbb{N} \tag{38}$$

<sup>11</sup> Applying this to  $m = q$ , we obtain  $a^{(p-1)q+1} \equiv a \pmod p$  (since  $q \in \mathbb{N}$ ). Multiplying both sides of this congruence with  $a^{r-1}$ , we find  $a^{(p-1)q+1}a^{r-1} \equiv aa^{r-1} = a^r \pmod p$ . Thus,

$$a^r \equiv a^{(p-1)q+1}a^{r-1} = a^{(p-1)q+1+(r-1)} = a^k \pmod p$$

---

<sup>11</sup>*Proof of (38):* We shall prove (38) by induction on  $m$ :

(since  $\underbrace{(p-1)q+1}_{=k-r} + (r-1) = k - r + 1 + (r-1) = k$ ). This proves Corollary 3.10. □

*Proof of Theorem 3.1.* If  $k < p - 1$ , then the claim of Theorem 3.1 follows from Lemma 3.8. Hence, for the rest of this proof, we WLOG assume that we don't have  $k < p - 1$ . Thus,  $k \geq p - 1 > 0$ . Hence,  $k$  is positive. Thus,  $k$  is not a multiple of  $p - 1$  (because  $k$  is not a positive multiple of  $p - 1$ , but is positive).

Let  $r$  be the remainder of  $k$  upon division by  $p - 1$ . Thus,  $r \in \{0, 1, \dots, (p - 1) - 1\}$ , so that  $r \in \mathbb{N}$  and  $r \leq (p - 1) - 1 < p - 1$ . Each  $l \in \{0, 1, \dots, p - 1\}$  satisfies  $l^k \equiv l^r \pmod p$  (by Corollary 3.10, applied to  $a = l$ ). Hence,

$$\sum_{l=0}^{p-1} \underbrace{l^k}_{\equiv l^r \pmod p} \equiv \sum_{l=0}^{p-1} l^r \equiv 0 \pmod p$$

(by Lemma 3.8, applied to  $r$  instead of  $k$ ). This proves Theorem 3.1. □

## References

- [Aigner07] Martin Aigner, *A Course in Enumeration*, Graduate Texts in Mathematics #238, Springer 2007.
- [AnBeRo05] Peter G. Anderson, Arthur T. Benjamin and Jeremy A. Rouse, *Combinatorial Proofs of Fermat's, Lucas's, and Wilson's Theorems*, The American Mathematical Monthly, Vol. 112, No. 3 (Mar., 2005), pp. 266–268.
- [BenQui03] Arthur T. Benjamin and Jennifer J. Quinn, *Proofs that Really Count: The Art of Combinatorial Proof*, The Mathematical Association of America, 2003.
- [Comtet74] Louis Comtet, *Advanced Combinatorics: The Art of Finite and Infinite Expansions*, D. Reidel Publishing Company, 1974.

*Induction base:* We have  $a^{(p-1)0+1} = a^1 = a \equiv a \pmod p$ . In other words, (38) holds for  $m = 0$ . This completes the induction base.

*Induction step:* Let  $n \in \mathbb{N}$ . Assume that (38) holds for  $m = n$ . We must prove that (38) holds for  $m = n + 1$ .

We have assumed that (38) holds for  $m = n$ . In other words,  $a^{(p-1)n+1} \equiv a \pmod p$ . Now,  $(p - 1)(n + 1) + 1 = ((p - 1)n + 1) + (p - 1)$ . Hence,

$$a^{(p-1)(n+1)+1} = a^{((p-1)n+1)+(p-1)} = \underbrace{a^{(p-1)n+1}}_{\equiv a \pmod p} a^{p-1} \equiv aa^{p-1} = a^p \equiv a \pmod p.$$

In other words, (38) holds for  $m = n + 1$ . This completes the induction step. Hence, (38) is proven.

- [GrKnPa] Ronald L. Graham, Donald E. Knuth, Oren Patashnik, *Concrete Mathematics, Second Edition*, Addison-Wesley 1994.
- [Grinbe16] Darij Grinberg, *Fleck's binomial congruence using circulant matrices*, 3 October 2018.  
<http://www.cip.ifi.lmu.de/~grinberg/fleck.pdf>
- [Grinbe17] Darij Grinberg, *Notes on the combinatorial fundamentals of algebra*, 4 October 2018.  
<https://github.com/darijgr/detnotes/releases/tag/2018-10-04>  
See also <http://www.cip.ifi.lmu.de/~grinberg/primes2015/sols.pdf> for a version that is getting updates.
- [Hausne83] Melvin Hausner, *Applications of a Simple Counting Technique*, The American Mathematical Monthly, Vol. 90, No. 2 (Feb., 1983), pp. 127–129.
- [Mestro14] Romeo Meštrović, *Lucas' theorem: its generalizations, extensions and applications (1878–2014)*, arXiv:1409.3820v1.
- [Stan11] Richard Stanley, *Enumerative Combinatorics, volume 1*, Second edition, version of 15 July 2011. Available at <http://math.mit.edu/~rstan/ec/>.
- [Stanto16] Dennis Stanton, *Addendum to "Using the "Freshman's Dream" to Prove Combinatorial Congruences"*,  
<http://www.math.rutgers.edu/~zeilberg/mamarim/mamarimhtml/freshmanDennisStanton.pdf>
-
